# Supplementary material for: Discovering Bias in Latent Space: An Unsupervised Debiasing Approach
Source: arXiv:2406.03631 source file (2024-06-05)
Supplement: Supplementary file 1 [file toxicity_results.tex]

\begin{table}[h]
    \centering
    \begin{tabular}{llcccc}
        \toprule
        \multirow{2}{*}{Model} & \multicolumn{2}{c}{Vanilla}& \multicolumn{2}{c}{\textbf{$\SYSNAME$}} \\ 
        \cmidrule(lr){2-3}  \cmidrule(lr){4-5}
        & AvgToxic($\downarrow$) & ROUGE-1($\uparrow$) & AvgToxic($\downarrow$) & ROUGE-1($\uparrow$) \\
        \toprule
        LLaVA & 0.053 & 76.19 & \textbf{0.049} & 75.34 \\
        IDEFICS & 0.082 & 85.44 & \textbf{0.074} & 84.08 \\
        InstructBLIP &  0.190 & 89.24 & \textbf{0.150} & 89.00 \\
        \bottomrule
    \end{tabular}
    \caption{Open Generation.}
    \label{tab:open_generation_exp}
\end{table}
We now provide an initial demonstration that $\SYSNAME$ can potentially work to reduce bias in open-ended generation tasks. Specifically, we test our technique for toxic word generation. The goal is to reduce the toxic generations.
\paragraph{Setup.} We use adversarial prompts dataset RealToxicityPrompts \cite{Gehman2020RealToxicityPromptsEN} to elicit toxic generation. We use the same prompt used by \cite{ilharco2022editing}. To find the direction corresponding to toxicity, we follow the same procedure as in Section \ref{sec:method}. We collect activation values by concatenating the prompt with words from HurtLex \cite{bassignana2018hurtlex}: a toxic words corpora.
\paragraph{Metrics.} We use the toxicity score generated by Detoxify \cite{Detoxify} and take the average across all generated sentences. To ensure the generated sentences are coherent with the given prompt, we also evaluate the similarity between the prompt and the resulting sentence post-generation using ROUGE-1 score \cite{lin-2004-rouge}.

\paragraph{Results.} Table \ref{tab:open_generation_exp} shows that using our simple training-free technique, it is possible to reduce toxicity scores of generated sentences elicited using crafted adversarial prompts while maintaining coherence to the prompt template.
